# Supplementary material for: An Identification and Dimensionality Robust Test for Instrumental Variables Models
Source: arXiv:2311.14892 source file (2024-12-14)
Supplement: Supplementary file 1 [file generated-lasso.tex]

\section{Consistency of LASSO with Generated Variables}
\label{sec:generated-lasso} 

In the below I will consider consistency results for the LASSO estimator with generated right hand side. Establishing consistency with generated left hand side variables follows from a symmetric proof. The parameter of interest is the conditional expectation \(y_i = \Pi(x_i) + e_i\) with \(\E[e_i|x_i] = 0\). I will assume that \(\Pi(x_i)\) has an approximately sparse representation in a basis \(b(x_i)\); \(\Pi(x_i) = b(x_i)'\pi + \xi_i\).
I will assume that the researcher does not directly observe \(b(x_i)\) but rather observes an estimate \(\hat b(x_i)\).

Consider two estimating problems;
\begin{align}
    \label{eq:infeasible-equation}
    \tilde\pi &= \arg\min_{\pi \in \SR^p} \frac{1}{2}\E_n[(y_i - b(x_i)'\pi)^2] + \lambda\|\pi\|_1 \\ 
    \label{eq:feasible-equation}
    \hat\pi &= \arg\min_{\pi \in \SR^p} \frac{1}{2}\E_n[(y_i - \hat b(x_i)'\pi)^2] + \lambda\|\pi\|_1
\end{align}
Standard LASSO consistency results will bound \(\|\tilde\pi-\pi\|_1\). In this section, I show that one can also bound \(\|\hat\pi - \tilde\pi\|_1\). To do so, I will need bounds on restricted and restricted sparse eigenvalues as in \citet{BC-2013}.  For any index set \(T \subseteq [p]\) define the vector \(\gamma_T \in \SR^p\) such that \((\gamma_T)_\ell = \gamma_\ell\) for \(\ell \in T\) and \((\gamma_T)_\ell = 0\) otherwise. For any \(c_0 > 1\) and \(T \subseteq p\) the restricted set is defined 
\[
    \Delta(c_0, T) = \{\gamma \in \SR^p : \|\gamma_{T^c}\|_1 \leq c_0\|\gamma_T\|_1, \gamma \neq 0\}
\]
Let \(S = \{j: \pi_j \neq 0\}\) denote the sparsity set and let \(s = |S|\) denote the true sparsity index. Define \(\Sigma \coloneqq \E_n[b(z)b(z)']\) and the restricted eigenvalue
\[
    \kappa^2(s \log(n), c_0) \coloneqq \min_{\substack{\gamma \in \Delta(c_0, T) \\ |T| \leq s\log(n)}} s\log(n) \frac{\gamma'\Sigma\gamma}{\|\gamma\|_1^2}
\]
The restricted sparse eigenvalue is defined 
\[
    \phi^2(m, T) \coloneqq \max_{\substack{\|\gamma_{T^c}\|_0 \leq m \\ \gamma \neq 0}} \frac{\gamma'\Sigma\gamma}{\|\gamma\|_2^2}
\]

\begin{assumption}[]
    \label{assm:generated-consistency}
    Assume there is a constant s.t 
\end{assumption}
\begin{prop}[]
    \label{prop:generated-consistency}
    
\end{prop}
\begin{proof}[Proof of \Cref{prop:generated-consistency}]
    The proof proceeds in three main steps. 

    \textbf{Step 1: Bound on Prediction Norm.}
    From the optimality of \(\tilde\pi\) in \eqref{eq:infeasible-equation} we have that, for any \(\bar\pi \neq \tilde\pi\) and any \(u \in (0,1]\):
    \begin{align*}
        \frac{1}{2}\E_n[(x - b(z)'\tilde\pi)^2] + \lambda\|\tilde\pi\|_1 
    \leq \frac{1}{2}\E_n[(x - b(z)'\{(1 - u)\tilde\pi + u\bar\pi\}\})^2] + \lambda\|(1 - u)\tilde\pi + u\bar\pi\|_1
    \end{align*}
    Using convexity of \(\|\cdot\|_1\) this yields
    \[
        \frac{1}{2}\E_n[(x - b(z)'\gamma)^2] - \frac{1}{2}\E_n[(x - b(z)'\{(1 - u)\tilde\pi + u\bar\pi\})^2] + u\lambda\|\tilde\pi\|_1 \leq u \lambda \|\bar\pi\|_1 
    \]
    Dividing both sides by \(u\) and letting \(u \to 0^+\) gives
    \[
        (\tilde\pi - \bar \pi)'\E_n[b(z_i)b(z_i)'](\tilde\pi - \bar\pi) + (\tilde\pi - \bar\pi)'\E_n[(x - b(z)'\pi)b(z)] + \lambda\|\tilde\pi\|_1 \leq \lambda\|\bar\pi\|_1
    \]
    Letting \(\delta = (\tilde\pi - \hat\pi)'\) and recalling the definition of \(\Sigma \coloneqq\E_n[b(z)b(z)']\)
    \begin{equation}
        \label{eq:infeasible-bound}
        \begin{split}
            \delta'\Sigma\delta + \delta'\E_n[(x - b(z)'\hat\pi)b(z)] + \lambda\|\tilde\pi\|_1
        \end{split}
    \end{equation}
    Repeating this analysis using the optimality of \(\hat\pi\) in \eqref{eq:feasible-equation} yields
    \begin{equation}
        \label{eq:feasible-bound}
        \begin{split}
            \delta'\Sigma\delta - \delta'\E_n[(x - \hat b(z)'\tilde\pi)\hat b(z)] + \lambda\|\hat\pi\|_1 \leq \lambda\|\tilde\pi\|_1
        \end{split}
    \end{equation}
    From \eqref{eq:feasible-bound} bound 
    \begin{align*}
        \lambda\|\hat\pi\|_1 
        &\leq \lambda\|\tilde\pi\|_1 + \delta'\E_n[(x - \hat b(z)'\tilde\pi)\hat b(z)] - \delta'\Sigma\delta \\ 
        &\leq \lambda\|\tilde\pi\|_1 + \delta'\E_n[(x - \hat b(z)'\pi)\hat b(z)] + \delta'\Sigma\delta \numberthis \label{eq:feasible-bound-rotated}
    \end{align*} 
    where in the second line we use that \(\Sigma\) is positive semi-definite. Plugging \eqref{eq:feasible-bound-rotated} into \eqref{eq:infeasible-bound} yields
\end{proof}
